# Supplementary material for: Making Theft Useless: Adulteration-Based Protection of Proprietary Knowledge Graphs in GraphRAG Systems
Source: arXiv:2601.00274 source file (2026-01-01)
Supplement: Supplementary file 1 [file artifact_appendix.tex]

% Artifact Appendix template for the NDSS Artifact Evaluation
% version 1.0 (20230620)

% remove the following block when merging the appendix with the camera-ready full paper
%%%
%\documentclass[conference]{IEEEtran}
%\pagestyle{plain}
%\usepackage{url}
%\begin{document}
%%%

\appendices
\section{Artifact Appendix}

The artifact appendix is meant to be a self-contained document presenting a roadmap for setting up and evaluating your artifact. It should provide the following elements:
\begin{enumerate}
\item a list of the hardware, software, and configuration \textbf{requirements} for running the artifact;
\item a clear description of how, and in what respects, the artifact \textbf{supports} the research presented in the paper;
\item a guide for how others can \textbf{execute and validate} the artifact for its functional and usability aspects;
\item the \textbf{major claims} made by your paper and a clear description of how to obtain data for each claim through your supplied artifact.
\end{enumerate}

Points 3-4 are not required if only the \textit{Available} badge is requested. Linking the paper claims to the artifact is a necessary step that allows artifact evaluators to functionally test and reproduce your results. Towards that end, explicitly list down items (e.g., results, plots, tables) from the paper and cross-reference them with the experiments to be reproduced.
 
Unless otherwise stated, filling every section below with the requested contents is mandatory for participating in the artifact evaluation process. Section titles cannot be changed.

\subsection{Description \& Requirements}

This section should list all the information necessary to recreate the experimental setup you used to run your artifact.

Provide also a link to an archival repository where all the artifact's main components (software, datasets, documentation, etc.) can be accessed and, where this applies, the minimal hardware and software requirements to run your artifact.

It is also very good practice to list and describe in this section benchmarks where those are part of your artifacts or simply have been used to produce results with it.

\subsubsection{How to access}
Describe here how to access your artifact. During the artifact evaluation, in case of a private repository, you should provide instructions on how to access it. For the camera-ready version of the appendix, you must provide a DOI link to the AEC-approved artifact version that you must upload by then to permanent storage.

\subsubsection{Hardware dependencies}
Simply write ``None." where this does not apply to your artifact.

\subsubsection{Software dependencies} 
Simply write ``None." where this does not apply to your artifact.

\subsubsection{Benchmarks} 
Describe here any data (e.g., datasets, models, workloads, etc.) required by the experiments with this artifact reported in your paper. Simply write ``None." where this does not apply to your artifact.

\subsection{Artifact Installation \& Configuration}

This section should include all the high-level installation and configuration steps required to prepare the environment to be used for the evaluation of your artifact.

\subsection{Experiment Workflow}

This section should provide a high-level view of the experimental workflow and how it is implemented, invoked, and (if needed) customized. The section is optional if the experiment workflow can be easily embedded in the Evaluation section.

\textit{Detailed information for submission, reviewing, and badging process followed for the evaluation of NDSS 2024 artifacts can be found at:} \url{https://secartifacts.github.io/ndss2024/}.

\subsection{Major Claims}
Enumerate here the major claims (Cx) made in your paper. For this purpose, we ask you to use the this and the following section and cross-reference the items therein, as explained next.

Follows an example:

\begin{itemize}
    \item (C1): \textsc{System} achieves the same accuracy of the state-of-the-art systems for a task X while saving 2x storage resources. This is proven by the experiment (E1) whose results are illustrated/reported in [refer to your paper's plots, tables, sections, etc.].
    \item (C2): \textsc{System} has been used to uncover new bugs in the Y software. This is proven by the experiments (E2) and (E3) in [ibid].
\end{itemize}

\subsection{Evaluation}

This section include all the operational steps and experiments which must be performed to evaluate if your artifact is functional and validate the proposed/presented experiments. For this purpose, we ask you to use the this and the preceding section and cross-reference the items therein.

If the \textit{Reproduced} badge is requested, the section should reference your paper's key results: describe the expected numbers and, where applicable, the maximum variation expected (particularly important for performance numbers). If an experiment is a scaled-down version of the one run for the paper's evaluation, provide a clear indication of it with a justification of the scaling-down being meaningful.

We also highly encourage you to provide your estimates of human- and compute-time for each of the listed experiments.

Follows an exemplary structure for one experiment (Ey):

\subsubsection{Experiment (E1)}
[Optional Name] [30 human-minutes + 1 compute-hour]: provide a short explanation of the experiment and expected results.

\textit{[How to]} Describe thoroughly the steps to perform the experiment and to collect and organize the results as expected from your paper. We encourage you to use the following structure with three blocks for the description of an experiment (and to provide precise indications about the expected outcome for each of the steps from the blocks):

\textit{[Preparation]}
Describe the steps required to prepare and configure the environment for this experiment.

\textit{[Execution]}
Describe the steps to run this experiment.

\textit{[Results]}
Describe the steps required to collect and interpret the results for this experiment.

\subsection{Customization}
Provide here notes on how to customize your experiments, when applicable. The section is optional.

\subsection{Notes}
This section is meant to allow authors to include any further important notes that may not fall within any of the previous categories. We kindly encourage you to remove this section where this sort of content may not be strictly needed (rather than filling it with unnecessary or redundant information).
