# Supplementary material for: Making Theft Useless: Adulteration-Based Protection of Proprietary Knowledge Graphs in GraphRAG Systems
Source: arXiv:2601.00274 source file (2026-01-01)
Supplement: Supplementary file 2 [file appendix_prompt_detect.tex]

\begin{promptbox}{Prompt for Extracting Triples}
\label{prompt_semantic_detect}
Act as an expert Knowledge Graph Analyst. Your task is to critically evaluate the semantic and factual validity of the following knowledge graph triple:

triple: \textcolor{red}{[triple]}

After performing a complete evaluation based on factual accuracy, type consistency, and common sense plausibility, provide a single-word response.

- Respond with `yes' ONLY if the triple is perfectly correct in every aspect.
- Respond with `no' if the triple fails for ANY reason.

Your entire response must be either `yes' or `no'. Do not provide any other text or explanation.
\end{promptbox}
